# Supplementary material for: Learn to Propagate Reliably on Noisy Affinity Graphs
Source: arXiv:2007.08802 source file (2020-07-17)
Supplement: Supplementary file 1 [file supp.tex]

% !TEX root = ../main.tex

\clearpage
